# Supplementary material for: Do the Findings of Document and Passage Retrieval Generalize to the Retrieval of Responses for Dialogues?
Source: arXiv:2301.05508 source file (2023-01-13)
Supplement: Supplementary file 1 [file appendix_resp2context_examples.tex]

\begin{table*}
\small
\caption{\textcolor{Brown}{Appendix B.} Random examples of augmentations by the \resptocontext{} methods.}
\label{table:resp2contex_examples}
\begin{tabular}{@{}p{1cm}p{6.5cm}p{2.5cm}p{3cm}p{3cm}@{}}
\toprule
Dataset & Context & Response & Augmentation \resptocontext{} & Augmentation \resptocontextlu{} \\ \midrule
\mantis{} & On macOs High Sierra I am trying to set a default icon for .pdf files: when I used Adobe Reader all the pdf files showed its icon, then I uninstalled it and replaced it with Foxit Reader as default app to open the same file. However all the pdf files now show a white icon and I would like them to show the Foxit logo instead.I tried to copy-paste the logo from Foxit to a random pdf and it does work, but this cannot be applied to the whole configuration (this means that I should copy-paste everytime the logo in every single pdf file).Is there a way to set the default icon? [UTT\_SEP] "Once you have changed the default application using Get Info, you may need to clear the icon cache.To get started, close all open applications and then launch Terminal from Macintosh HD > Applications > Utilities. Copy and paste the following command at the Terminal prompt and press Return to execute it: [code removed for paper] Restart, job done.From [URL] Safari download bar rar file icon show as VLC icon,which associate to The Unarchiver should shows its icon" [UTT\_SEP] I did what you explained but the problem still exist. I have updated to Mojave since the last time. In Finder (choosing the list view for my files) I still see .pdf icon represented as a blank page. & It appears Foxit Reader is missing the readerpdf.icns file. As a quick fix until the developer releases a solution you could borrow the PDF icon from another app or find an icon from a previous version. & The newest version of Foxit Reader is , which comes with Firefox, and has an icon for Adobe PDF Reader.  is a version that was released by Foxit in May of 2014. However, this is not an update, it has been updated to a different version.  is in a separate file that the reader PDF icon can be found in a new window and it is a  PDF icon a new icon is found on the new window and not the app store. I have not been [...] & I tried it and it worked. I just reinstalled the software and the app works fine. I have to say that i can't find a PDF icon. I've renamed and downloaded the app. \\ \midrule
\msdialog{} & KF-UK you are not alone. What I did, is I uninstalled all new updates and paused the download feature. Hopefully someone has a workaround before serious problems occur. As you know Microsoft is a security conscious organization looking out for the well being of it customers. In other words we need your money but if the matter hits the fan we have no knowledge of your existence but would you recommend our products to your friends.   [UTT\_SEP]  Even after KB4040724 (build 15063.632) update, the issue persists (in my case). There are two workaround for this issue reguarding my opinion at the moment: 1 - at login or later, the combination of shift-ctrl-win + B restores the graphics card and this ""awaken"" the monitor in standby 2 - Turn off Fast Boot by disabling it via Control Panel \ Power Options \ Choose What the Power Buttons do \ Change Settings that are Currently Unavailable \ untick ""Turn on fast startup"". & I too am having problems with a dual monitor setup. My system had KB4038788 installed this month. I will attempt an uninstall and see if the dual monitor sleep issue goes away.... Complete symptom details for me are below. I am subscribing to this thread hoping Microsoft provides an answer. & My 870 has been working great and my 810 is having some problems (like the aforementioned one). Is this an update that is supposed to fix the 870, which I'm not sure I'm missing - I'm not sure what happened and if I'm not a 870, I'm not a 870. I don't know what happened and it just hangs up in bed [...] & for your reply. I have the same problem as you, if I am on my iMac. When I wake up, it will go to sleep but when I get up to do that the same thing happens again. It's also not the same. I'm using the 2nd monitor. I've also slept well on this monitor for 2 years, so it' \\ \midrule
\ubuntu{} & anyone notices there is something wrong with man page of netstat..... [UTT\_SEP] wondering if its only me... or there is something wrong [UTT\_SEP] it looks fine to me [UTT\_SEP] my man page is not showing argument options, like -an etc & mine shows both -a and -n :\ & Hello, a lot of ubuntu users have asked me this on the forum, and I just can't seem to figure this out, but when I open my terminal, it asks me ""Can I do anything with my ubuntu"?" [UTT\_SEP] how [...] & how to change the name of a pc in gnome-server? \\ \bottomrule
\end{tabular}
\end{table*}
