# Supplementary material for: Do the Findings of Document and Passage Retrieval Generalize to the Retrieval of Responses for Dialogues?
Source: arXiv:2301.05508 source file (2023-01-13)
Supplement: Supplementary file 2 [file appendix_rm3.tex]

% Please add the following required packages to your document preamble:
% \usepackage{booktabs}
\begin{table*}[hbt!]
\small
\caption{\textcolor{Brown}{Appendix A.} Hyperparameters tested for RM3. The hyperparameters are: number of expansion terms - number of expansion documents - weight to assign to the original query. We see that when we use more of the original query we get higher effectiveness and other hyperparameters do not help much either decreasing or increasing.}
\label{table:rm3_results}
\begin{tabular}{@{}lllllll@{}} % 
\toprule
                               & \multicolumn{2}{l}{\textbf{\mantis{}}} & \multicolumn{2}{l}{\textbf{\msdialog{}}} & \multicolumn{2}{l}{\textbf{\ubuntu{}}} \\ \midrule
                               & \textbf{R@1}       & \textbf{R@10}     & \textbf{R@1}        & \textbf{R@10}      & \textbf{R@1}       & \textbf{R@10}     \\ \midrule
\bm{} & \textbf{0.133} & \textbf{0.299} & \textbf{0.064} & \textbf{0.177} & \textbf{0.027} & \textbf{0.070} \\ \hdashline
+\rmthree{} (5-5-0.5) & 0.089 & 0.214 & 0.042 & 0.133 & 0.014 & 0.042 \\
+\rmthree{} (5-5-0.7) & 0.097 & 0.238 & 0.048 & 0.150 & 0.017 & 0.051 \\
+\rmthree{} (5-10-0.5) & 0.072 & 0.190 & 0.036 & 0.123 & 0.010 & 0.037 \\
+\rmthree{} (5-10-0.7) & 0.086 & 0.218 & 0.043 & 0.145 & 0.012 & 0.047 \\
+\rmthree{} (5-15-0.5) & 0.066 & 0.175 & 0.032 & 0.115 & 0.008 & 0.038 \\
+\rmthree{} (5-15-0.7) & 0.080 & 0.206 & 0.039 & 0.135 & 0.010 & 0.047 \\
+\rmthree{} (10-5-0.5) & 0.094 & 0.248 & 0.042 & 0.150 & 0.016 & 0.053 \\
+\rmthree{} (10-5-0.7) & 0.103 & 0.266 & 0.048 & 0.161 & 0.019 & 0.058 \\
+\rmthree{} (10--10-0.5) & 0.081 & 0.221 & 0.038 & 0.136 & 0.014 & 0.049 \\
+\rmthree{} (10-10-0.7) & 0.092 & 0.246 & 0.046 & 0.153 & 0.015 & 0.057 \\
+\rmthree{} (10-15-0.5) & 0.073 & 0.206 & 0.035 & 0.127 & 0.011 & 0.049 \\
+\rmthree{} (10-15-0.7) & 0.085 & 0.232 & 0.044 & 0.142 & 0.017 & 0.056 \\
+\rmthree{} (15-5-0.5) & 0.099 & 0.261 & 0.045 & 0.152 & 0.019 & 0.057 \\
+\rmthree{} (15-5-0.7) & 0.107 & 0.275 & 0.050 & 0.162 & 0.022 & 0.061 \\
+\rmthree{} (15--10-0.5) & 0.085 & 0.238 & 0.036 & 0.145 & 0.013 & 0.054 \\
+\rmthree{} (15-10-0.7) & 0.097 & 0.258 & 0.048 & 0.156 & 0.016 & 0.059 \\
+\rmthree{} (15-15-0.5) & 0.077 & 0.219 & 0.036 & 0.131 & 0.014 & 0.054 \\
+\rmthree{} (15-15-0.7) & 0.091 & 0.245 & 0.042 & 0.148 & 0.017 & 0.060 \\ \bottomrule
\end{tabular}
\end{table*}
